# Supplementary material for: ENTP: Encoder-only Next Token Prediction
Source: arXiv:2410.01600 source file (2025-02-04)
Supplement: Supplementary file 1 [file additional-nlp-experiments.tex]

In this section, we present additional experimental results for natural language processing (NLP) tasks, comparing the performance of a decoder-only model and an ENTP, both trained on OpenWebText~\citep{Gokaslan2019OpenWeb}, as discussed in \Cref{sec:openwebtext}.

First, we evaluated commonsense reasoning ability using the TinyWinoGrande benchmark~\citep{tinybenchmarks}, which involves identifying the referents of pronouns. After pre-training on OpenWebText, both models were evaluated on this benchmark in a zero-shot manner. As shown in the \Cref{tab:tinywino}, ENTP achieved higher accuracy than the decoder-only model, highlighting its potential effectiveness  across diverse downstream tasks.

Next, we evaluated the models on an NLP classification task using the CLUTRR dataset~\citep{CLUTRR}. This reasoning-based dataset is designed to classify relationships between individuals based on textual descriptions. Both models, pre-trained on OpenWebText, were fine-tuned on limited subsets of the CLUTRR data. 
The results are presented in Figure~\ref{fig:clutrr}. We note that their performance was then evaluated on a separate holdout dataset. 

\begin{table*}[htpb]
    \centering
    \caption{The performance of Decoder-only model and ENTP on TinyWinoGrande benchmark.}
    \resizebox{0.5\linewidth}{!}
    {
    \begin{tabular}{lcc}
    \toprule
     & Decoder-only & Encoder-only (ENTP) \\
    \midrule
    Accuracy & 56.0 \%	& 61.0 \% \\
    \bottomrule
    \end{tabular}
    }
    \label{tab:tinywino}
\end{table*}

\begin{figure}[htbp]
    \centering
    \includegraphics[width=.5\linewidth]{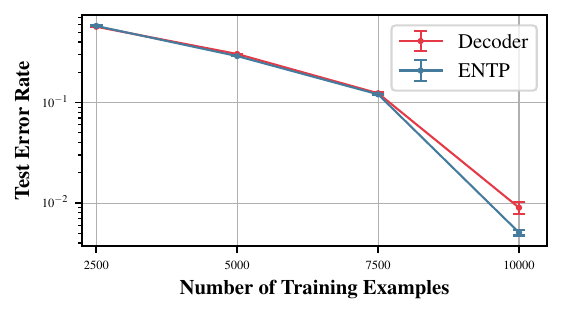}
    \vspace{-1em}
    \caption{We fine-tune the models trained on OpenWebText to perform the CLUTRR task \citep{CLUTRR}. We find that ENTP either outperforms or matches the performance of decoder.}
    \label{fig:clutrr}
\end{figure}
