# Supplementary material for: ENTP: Encoder-only Next Token Prediction
Source: arXiv:2410.01600 source file (2025-02-04)
Supplement: Supplementary file 2 [file triplet.tex]

In this section, we conducted $\operatorname{Count3}$ experiments with additional Transformer variants. First, we evaluated the performance of Prefix decoder-only models~\citep{T5, wu2021yuan}, which perform non-causal attention for the prefix portion. Using the same experimental setup, we initiated sequences with 16 random seeds, which were used as the prefix. As shown in Figure ~\ref{fig:added_triplet}, while the Prefix decoder-only model slightly outperforms the decoder-only model, it also fails to learn the triplet counting task. This demonstrates that performing full attention to certain parts of a sequence in a decoder-only model is insufficient to solve tasks requiring $\operatorname{Count3}$-level complexity.

Next, we conducted experiments on the $\operatorname{Count3}$ task using BERT~\citep{devlin2019bertpretrainingdeepbidirectional}, a representative encoder-only architecture. Specifically, we fine-tuned BERT using the ENTP approach under the same experimental conditions. As shown in Figure~\ref{fig:added_triplet}, BERT combined with ENTP successfully learned triplet counting. Notably, as BERT is pre-trained and larger compared to the medium transformer used in the paper, it converged more quickly. This result indicates that ENTP is effective not only for the model configurations specified in the main paper but also for larger pre-trained models.

\begin{figure}[h]
    \centering
    \includegraphics[width=1.0\linewidth]{figures/triplet_bert_prefix.pdf}
    \vspace{-1em}
   \caption{The performance of the Prefix decoder-only model and BERT combined with ENTP on the Count3 task.}
    \label{fig:added_triplet}
    % \vspace{-1em}
\end{figure}
